# Supplementary material for: I Still See You: Why Existing IoT Traffic Reshaping Fails
Source: arXiv:2406.10358 source file (2024-06-14)
Supplement: Supplementary file 1 [file appendix.tex]

\section{Additional User Activities Visualization and Image-based Attack Results}
\label{sec:set-diff-dodis}

\begin{figure*}[htbp]
\centering              
\begin{tabular}{cccc}       
\includegraphics[width=0.3\textwidth]{./Qi/activities/0_07_32.pdf} &
\includegraphics[width=0.3\textwidth]{./Qi/activities/1_01_468.pdf}& 
\includegraphics[width=0.3\textwidth]{./Qi/activities/2_01_303.pdf} \\
0 &  1  & 2 \\
\includegraphics[width=0.3\textwidth]{./Qi/activities/3_01_1249.pdf}&
\includegraphics[width=0.3\textwidth]{./Qi/activities/4_01_947.pdf} &
\includegraphics[width=0.3\textwidth]{./Qi/activities/5_01_1438.pdf} \\
3 &  4  & 5 \\

\includegraphics[width=0.3\textwidth]{./Qi/activities/6_01_1339.pdf} &
\includegraphics[width=0.3\textwidth]{./Qi/activities/7_01_1315.pdf} &
\includegraphics[width=0.3\textwidth]{./Qi/activities/8_01_1327.pdf} \\
 6 & 7 & 8  \\

\includegraphics[width=0.3\textwidth]{./Qi/activities/9_06_1406.pdf} &
\includegraphics[width=0.3\textwidth]{./Qi/activities/10_04_1065.pdf} &
\includegraphics[width=0.3\textwidth]{./Qi/activities/11_07_193.pdf} \\

9 &  10  & 11  \\
\includegraphics[width=0.3\textwidth]{./Qi/activities/12_08_344.pdf} &
\includegraphics[width=0.3\textwidth]{./Qi/activities/13_01_1176.pdf} \\
12 &  13 \\

\end{tabular}
\caption{The visualization of 14 user activities.}
\label{fig:activities_visualization}
\vspace{-0.5cm}
\end{figure*}

\begin{table*}[t!]
\small
\begin{center}
\begin{tabular}{||c|c|c|c||}
\hline
    \textbf{Activity ID} & \textbf{Devices}  & \textbf{Frequency} \\ \hline
         0  & InsteonCam (In)	 &	2616 \\ \hline
        1 & Amazon (In), Amazon (Out)	 &	956 \\ \hline
       2   &  BabyMonitor (Out)	 &844	 \\ \hline   
       3  & Amazon (In)	 &	711 \\ \hline
      4  & PhotoFrame (In)		 &	689 \\ \hline
        5 &  TPLinkCam (In)		 &	484 \\ \hline
        6 &  TPLinkCam (In)	, TPLinkCam (Out) 		 & 376	 \\ \hline
        7 &  DropCam (Out)	 &298	 \\ \hline
        8 & TPLinkCam (In), DropCam (Out), TPLinkCam (Out)		 &	228 \\ \hline
        9 & SleepSensor (Out)		 & 163	 \\ \hline
       10  & BelkinPlug (In)  &	139	 \\ \hline
       11  & Amazon (In), InsteonCam (In), Amazon (Out)		 &	126 \\ \hline
       12  & InsteonCam (In), BabyMonitor (Out)  &	117	 \\ \hline
       13  & 	BabyMonitor (In)  &	116 \\ \hline
   
\end{tabular}
\end{center}
\caption{The list of all the user activities when applying background filter as of 2,000 KB/S.}
\label{table:a-all-activity}
\end{table*}

% \begin{table*}[t!]
% %\small
% \begin{center}
% \begin{tabular}{||c|c|c|c||}
% \hline
%     \textbf{Activity Number} & \textbf{Devices} & \textbf{Activities }  & \textbf{Frequency} \\ \hline
%          0  & InsteonOut	& 	 &	681 \\ \hline
%         1 & InsteonIn, InsteonOut	& 	 &	529 \\ \hline
%        2   &  DropcamOut	&  & 475	 \\ \hline   
%        3  & WeatherIn	& 	 &	354 \\ \hline
%       4  & AmazonIn, AmazonOut	& 	 &	339 \\ \hline
%         5 &  InsteonOut, DropcamOut	& 	 &	313 \\ \hline
%         6 &  AmazonIn, AmazonOut, InsteonOut 	& 	 & 263	 \\ \hline
%         7 &  InsteonIn, InsteonOut, DropcamOut	& 	 &	257 \\ \hline
%         8 & SpeakerIn, SpeakerOut	& 	 &	230 \\ \hline
%         9 & SpeakerIn, SpeakerOut, InsteonOut	& 	 & 227	 \\ \hline
%        10  & WeatherIn, InsteonOut	&  &	216	 \\ \hline
%        11  & LIFXIn, InsteonOut	& 	 &	190 \\ \hline
%        12  & WeatherIn, DropcamOut	&  &	189	 \\ \hline
%        13  & 	AmazonIn, InsteonIn, AmazonOut, InsteonOut & 	 &	178 \\ \hline
%        14 & 	WeatherIn, InsteonIn, InsteonOut & 	 & 176	 \\ \hline
%     15 & AmazonIn, AmazonOut, DropcamOut	 & 	 &	161 \\ \hline
%         16 & AmazonOut, InsteonOut	 & 	 &	159 \\ \hline
%           17 & InsteonOu,sleepOut	 & 	 &	153 \\ \hline
%          18 & AmazonIn, WeatherIn, AmazonOut	 & 	 & 136	 \\ \hline
%         19  & InsteonIn, AmazonOut, InsteonOut	 & 	 & 125	 \\ \hline
        
% \end{tabular}
% \end{center}
% \caption{Activities labeling, threshold = 500, different thresholds, different motif frequency. There are other thresholds' graphs, and I can upload them if needed. }
% \end{table*}

\begin{table*}
\small
\begin{center}
\begin{tabular}{||c|c|c|c|c|c|c||}
\hline
    \textbf{Devices Activity} & \textbf{Top 1} & \textbf{Top 5} & \textbf{MCC} & \textbf{Precision} & \textbf{REcall} & \textbf{F1 score}\\ \hline
% Thresholding &15.47\%	   &94.62\%  & 5.38\%    &84.53\%  &0.06 \\ \hline
       all  & 79.1\%	& 96.0\%	& 0.722	& 0.794	& 0.790&0.781 \\ \hline
        0 & 88.8\%	& 98.5\%	& 0.734	& 0.771& 0.888 &0.825 \\ \hline
        1 & 86.1\%	& 97.2\%	& 0.787	& 0.770	& 0.861 & 0.813 \\ \hline
        10 & 31.8\%	& 72.7\%	& 0.262& 0.241	& 0.318 & 0.275\\ \hline
        11 & 15.0\%& 100\%	& 0.385	& 1.000	& 0.150 & 0.261 \\ \hline
        12 & 31.6\%	& 89.5\%	& 0.324	& 0.353	& 0.316 & 0.333 \\ \hline
        13 & 72.2\%	& 94.4\%	& 0.763	& 0.813	& 0.722 & 0.765 \\ \hline
        2 & 94.5\%	& 98.4\%	& 0.899	& 0.877	& 0.945&0.910 \\ \hline
        3 & 63.9\%	& 93.5\%	& 0.632	& 0.690	& 0.639 &0.663 \\ \hline
        4 & 51.0\%	& 87.5\%	& 0.539	& 0.646	& 0.510 & 0.570\\ \hline
        5 & 29.7\%	& 81.1\%	& 0.389	& 0.579	& 0.297 & 0.393 \\ \hline
        6 & 84.2\%	& 98.2\%	& 0.876	& 0.923	&0.842 & 0.881  \\ \hline
        7 & 80.4\%	& 95.7\%	& 0.806	& 0.822	& 0.804 &0.813 \\ \hline
        8 & 91.4\%	& 100\%	& 0.862	&0.821	& 0.914 & 0.865\\ \hline
        9 & 48.0\%	& 92.0\%	& 0.528	& 0.600	&0.480& 0.533 \\ \hline
        
\end{tabular}
\end{center}
\caption{The accuracy comparison of image-based attack on original protected network traffic rate data.}
\end{table*}

\begin{table*}
\small
\begin{center}
\begin{tabular}{||c|c|c|c|c|c|c||}
\hline
    \textbf{Devices Activity} & \textbf{Top 1} & \textbf{Top 5} & \textbf{MCC} & \textbf{Precision} & \textbf{REcall} & \textbf{F1 score}\\ \hline
% Thresholding &15.47\%	   &94.62\%  & 5.38\%    &84.53\%  &0.06 \\ \hline
       all  & 53.1\%	& 84.7\%	& 0.495	& 0.481	& 0.531&0.493 \\ \hline
        0 & 79.9\%	& 98.7\%	& 0.485	& 0.579& 0.799 &0.672 \\ \hline
        1 & 56.9\%	& 80.6\%	& 0.485 & 0.590	& 0.569	& 0.580  \\ \hline
        10 & 0.0\%	& 54.5\%	& 0 & 0	& 0 & 0\\ \hline
        11 & 0.0\%  & 25.0\%	& 0	& 0	& 0 & 0 \\ \hline
        12 & 0.0\%	& 42.1\%	& 0	& 0	& 0 & 0 \\ \hline
        13 & 5.6\%	& 27.8\%	& 0.081	& 0.143	& 0.056 & 0.080 \\ \hline
        2 & 55.5\%	& 83.6\%	& 0.512	& 0.573	& 0.555 & 0.564 \\ \hline
        3 & 28.7\%	& 75.0\%	& 0.342	& 0.517	& 0.287 & 0.369 \\ \hline
        4 & 33.7\%	& 87.5\%	& 0.282	& 0.350	& 0.337 & 0.343\\ \hline
        5 & 5.4\%	& 81.1\%	& 0.068	& 0.182	& 0.054 & 0.083 \\ \hline
        6 & 66.7\%	& 86.0\%	& 0.584	& 0.551	& 0.667 & 0.603  \\ \hline
        7 & 76.1\%	& 93.5\%	& 0.568	& 0.455	& 0.761 & 0.569 \\ \hline
        8 & 57.1\%	& 97.1\%	& 0.577	& 0.606	& 0.571 & 0.588\\ \hline
        9 & 12.0\%	& 48.0\%	& 0.147	& 0.214	& 0.120 & 0.154 \\ \hline
        
\end{tabular}
\end{center}
\caption{The accuracy comparison of image-based attack on PrivacyGuard~\cite{PrivacyGuard} protected network traffic rate data.}
\end{table*}

\begin{table*}
\small
\begin{center}
\begin{tabular}{||c|c|c|c|c|c|c||}
\hline
    \textbf{Devices} & \textbf{Top 1} & \textbf{Top 5} & \textbf{MCC} & \textbf{Precision} & \textbf{Recall} & \textbf{F1 score}\\ \hline
% Thresholding &15.47\%	   &94.62\%  & 5.38\%    &84.53\%  &0.06 \\ \hline
        all     & 68.1\%    & 93.1\% & 0.414 & 0.665 & 0.681 & 0.667 \\ \hline
        Withings Sleep Sensor   & 55.6\%	& 77.7\%	& 0.640	& 0.757	& 0.558 & 0.642 \\ \hline
        Amazon Echo Dot  & 81.2\%	& 96.8\%	& 0.784 & 0.837	& 0.813 & 0.822\\ \hline
        Dropcam Camera & 87.4\%    & 98.8\%	& 0.740	& 0.732	& 0.874 & 0.797 \\ \hline
        Insteon Camera & 64.7\%	& 97.4\%	& 0.507	& 0.518	& 0.647 & 0.575 \\ \hline
        Samsung Smart Camera & 5.3\%	    & 26.3\%	& 0.100	& 0.200	& 0.053 & 0.083 \\ \hline
        Belkin Motion Sensor  & 41.2\%	& 88.6\%	& 0.397	& 0.470	& 0.412 & 0.439 \\ \hline
        Withings Baby Monitor    & 53.6\%	& 86.6\%	& 0.518	& 0.602	& 0.548 & 0.674\\ \hline
        TP-Link Camera     & 90.8\%	& 96.6\%	& 0.922	& 0.941	& 0.908 & 0.924 \\ \hline
        HP Printer & 0\%	    & 28.6\%	& 0	& 0	& 0 & 0  \\ \hline
        Belkin Switch  & 0\%	& 22.2\%	& 0	& 0	& 0 & 0 \\ \hline
        Belkin Plug    & 11.4\%	& 43.2\%	& 0.160	& 0.250	& 0.114 & 0.156 \\ \hline
        Netatmo Camera & 66.0\%	& 89.0\%    & 0.624	& 0.695	& 0.660	& 0.677 \\ \hline
        Triby Speaker & 0\%	& 20\%	& 0	& 0	&0 &0  \\ \hline
        Pix-Star Photo Frame   & 45.5\%	& 81.4\%	& 0.450	& 0.510	& 0.455 & 0.481 \\ \hline
\end{tabular}
\end{center}
\caption{The accuracy comparison of image-based device event attack on PrivacyGuard~\cite{PrivacyGuard} protected network traffic rate data.}
\end{table*}

\begin{table*}
\small
\begin{center}
\begin{tabular}{||c|c|c|c|c|c|c||}
\hline
    \textbf{Devices} & \textbf{Top 1} & \textbf{Top 5} & \textbf{MCC} & \textbf{Precision} & \textbf{Recall} & \textbf{F1 score}\\ \hline
% Thresholding &15.47\%	   &94.62\%  & 5.38\%    &84.53\%  &0.06 \\ \hline
       all  & 87.2\%	& 97.4\%	& 0.643	& 0.865	& 0.872&0.867 \\ \hline
        % Tab & 93.8\%	& 100\%	& 0.904	& 0.882	& 0.938 &0.909 \\ \hline
        Withings Sleep Sensor & 88.1\%	& 97.0\%	& 0.878	& 0.881	& 0.846 & 0.917 \\ \hline
        Amazon Echo Dot & 96.4\%	& 98.8\%	& 0.924& 0.935	& 0.963 & 0.949\\ \hline
        Dropcam Camera & 89.3\%& 98.6\%	& 0.863	& 0.874	& 0.893 & 0.883 \\ \hline
        % scale & 100\%	& 100\%	& 1.00	& 1.000	& 1.000 & 1.000 \\ \hline
        Insteon Camera & 88.7\%	& 96.9\%	& 0.837	& 0.837	& 0.887 & 0.861 \\ \hline
        Samsung Smart Camera & 6.7\%	& 83.3\%	& 0.127	& 0.250	& 0.667&0.105 \\ \hline
        Belkin Motion Sensor & 69.8\%	& 97.4\%	& 0.705	& 0.743	& 0.698 &0.720 \\ \hline
        Withings Baby Monitor & 87.6\%	& 98\%	& 0.874	& 0.890	& 0.872 & 0.881\\ \hline
        TP-Link Camera & 95.2\%	& 98.4\%	& 0.921	& 0.894	& 0.952 & 0.923 \\ \hline
        HP Printer & 33\%	& 84\%	& 0.332	& 0.333	&0.456 & 0.333  \\ \hline
        Belkin Switch & 42.4\%	& 85.7\%	& 0.566	& 0.750	& 0.429 &0.545 \\ \hline
        % Things & 100\%	& 100\%	& 0.972	&0.947	& 1.000 & 0.973\\ \hline
        Belkin Plug & 46.9\%	& 81.2\%	& 0.515	& 0.577	& 0.469& 0.517 \\ \hline
        % Weather & 100\%	& 100\%	& 1.00	& 1.000	& 1.000& 1.000 \\ \hline
        % LIFX & 92.3\%	& 100\%	& 0.959	& 1.000	& 0.923 & 0.960 \\ \hline
        Netatmo Camera & 84.4\%	& 96.4\%&0.828	& 0.868	& 0.844	& 0.856 \\ \hline
        Triby Speaker & 20.0\%	& 86.7\%	& 0.271	& 0.375	&0.200&0.261  \\ \hline
        Pix-Star Photo Frame & 67.8\%	& 88.1\%	& 0.690	& 0.727	& 0.678& 0.702 \\ \hline
\end{tabular}
\end{center}
\caption{The accuracy comparison of image-based device event attack on original network traffic rate data.}
\end{table*}

\begin{table*}[t!]
\small
\begin{center}
\begin{tabular}{||c|c|c|c|c|c|c|c||}
\hline
    \textbf{Data} & \textbf{Image} & \textbf{Top\_1 Accuracy} & \textbf{Top\_5 Accuracy }  & \textbf{ MCC} & \textbf{ Precision} & \textbf{ Recall} & \textbf{ F1 Score}\\ \hline
       Original  & Line Chart  & 85.2\%	& 	96.6\% &	0.643 & 0.787 & 0.594&0.679 \\ \hline
       Original & Heat Map & 87.2\% & 97\%	 &	0.643 & 0.739 & 0.631 & 0.699\\ \hline
      Original & Scatter Plot   & 71.8\%	& 90.4\% & 0.506 & 0.753 & 0.570& 0.698\\ \hline   
      Original  & GAF & 66.2\%	& 94.6\%&	0.314 & 0.379 & 0.323&0.332\\ \hline
      RTP  & Line Chart & 69.6\%	& 91.3\%&	0.453 &0.523  & 0.456& 0.547\\ \hline
      RTP  & Heat Map & 73.1\%	& 93.5\%&	0.503 & 0.577 & 0.495& 0.515\\ \hline
      RTP  & Scatter Plot & 63.2\%	& 98.7\%&	0.505 & 0.587 & 0.500& 0.527\\ \hline
      RTP  & GAF & 62.9\%	& 93.8\%&	0.348 & 0.631 & 0.362& 0.573\\ \hline
      HTR  & Line Chart & 65.9\%	& 88.0\%&	0.411 & 0.472 &0.417 & 0.433\\ \hline
      HTR  & Heat Map & 68.9\%	& 93.0\%&	0.431 & 0.611 & 0.441& 0.573\\ \hline
      HTR  & Scatter Plot & 54.9\%	& 89.8\%& 0.395&0.636 & 0.378& 0.430 \\ \hline
      HTR  & GAF & 48.8\%	& 89.1\%&	0.232 & 0.297 & 0.262&0.264\\ \hline
      PrivacyGuard  & Line Chart & 66.4\%& 93.3\%&	0.372 & 0.418 & 0.388& 0.396\\ \hline
      PrivacyGuard  & Heat Map & 68.1\%	& 93.0\%&	0.414 & 0.465 & 0.429& 0.434\\ \hline
      PrivacyGuard  & Scatter Plot & 59.8\%	& 89.6\%&	0.567 &0.561  & 0.393& 0.418\\ \hline
      PrivacyGuard  & GAF & 54.7\%	& 92.0\%&	0.278 & 0.589 & 0.290& 0.450\\ \hline
      
\end{tabular}
\end{center}
\caption{The comparison of image representation based IoT device event attack.}
% \vspace{-0.2cm}
\end{table*}

\begin{figure*}[t!]
\centering              
\includegraphics[width=0.8\textwidth]{./Source/Su/confusion_matrix_original_pg.png}
\caption{The image-base attack confusion matrix on network traces modified by PrivacyGuard~\cite{PrivacyGuard} defense.}
\label{fig:confusion-matrix}
% \vspace{-0.2cm}
\end{figure*}
